# Supplementary material for: CoShNet: A Hybrid Complex Valued Neural Network using Shearlets
Source: arXiv:2208.06882 source file (2022-10-29)
Supplement: Supplementary file 1 [file appendix.tex]

\section{Appendix}
%The appendix section was placed after conclusion and before references in "Deep scattering spectrum" by J Anden and Mallat.

\subsection{Some Interesting Experiments}
Some interesting experiments which do not contribute to the central message of the paper but provide interesting results regardless are provided herein.
